# Supplementary material for: A case for using rotation invariant features in state of the art feature matchers
Source: arXiv:2204.10144 source file (2022-07-03)
Supplement: Supplementary file 1 [file supplementary.tex]

\appendix
